# Supplementary material for: On the Coexistence and Ensembling of Watermarks
Source: arXiv:2501.17356 source file (2025-01-29)
Supplement: Supplementary file 1 [file appendix_results.pdf]

| First method | Second method      | ECC          | Ensemble | Clip | Capacity<br>(bits) | Accuracy | Mean<br>PSNR [dB] | Std<br>PSNR [dB] | Robust.<br>RivaGAN | Robust.<br>SSL | Robust.<br>TmLow | Robust.<br>TmMed | Robust.<br>TmHigh |
|--------------|--------------------|--------------|----------|------|--------------------|----------|-------------------|------------------|--------------------|----------------|------------------|------------------|-------------------|
| DwtDet       | DwtDet             | -            | parallel | 0.5  | 64                 | 0.0%     | 38.7              | 4.1              | 0.0%               | 0.0%           | 0.0%             | 0.0%             | 0.0%              |
| DwtDet       | DwtDet             | -            | parallel | -    | 64                 | 0.0%     | 38.7              | 4.1              | 0.0%               | 0.0%           | 0.0%             | 0.0%             | 0.0%              |
| DwtDet       | DwtDet             | -            | series   | 0.5  | 64                 | 0.0%     | 40.7              | 2.3              | 0.0%               | 0.0%           | 0.0%             | 0.0%             | 0.0%              |
| DwtDet       | DwtDet             | -            | series   | -    | 64                 | 0.0%     | 40.5              | 2.2              | 0.0%               | 0.0%           | 0.0%             | 0.0%             | 0.0%              |
| DwtDet       | DwtDetSvd          | -            | parallel | 0.5  | 64                 | 10.0%    | 39.4              | 4.5              | 2.9%               | 0.9%           | 0.0%             | 0.0%             | 0.0%              |
| DwtDet       | DwtDetSvd          | -            | parallel | -    | 64                 | 10.0%    | 39.4              | 4.5              | 2.5%               | 1.3%           | 0.0%             | 0.0%             | 0.0%              |
| DwtDet       | DwtDetSvd          | -            | series   | 0.5  | 64                 | 52.9%    | 39.8              | 2.5              | 12.6%              | 5.8%           | 0.0%             | 0.0%             | 0.0%              |
| DwtDet       | DwtDetSvd          | -            | series   | -    | 64                 | 57.2%    | 39.1              | 2.0              | 13.3%              | 6.4%           | 0.0%             | 0.0%             | 0.0%              |
| DwtDet       | HiDDeN             | -            | parallel | 0.5  | 80                 | 0.2%     | 37.2              | 3.9              | 0.0%               | 0.0%           | 0.0%             | 0.0%             | 0.0%              |
| DwtDet       | HiDDeN             | -            | parallel | -    | 80                 | 0.2%     | 37.0              | 4.0              | 0.0%               | 0.0%           | 0.0%             | 0.0%             | 0.0%              |
| DwtDet       | HiDDeN             | -            | series   | 0.5  | 80                 | 0.6%     | 35.5              | 3.5              | 0.0%               | 0.0%           | 0.0%             | 0.0%             | 0.0%              |
| DwtDet       | HiDDeN             | -            | series   | -    | 80                 | 6.9%     | 32.0              | 4.1              | 1.8%               | 1.1%           | 0.0%             | 0.0%             | 0.0%              |
| DwtDet       | -                  | -            | -        | -    | 32                 | 51.0%    | 38.3              | 3.8              | 12.7%              | 6.4%           | 0.0%             | 0.1%             | 0.0%              |
| DwtDet       | RivaGAN            | -            | parallel | 0.5  | 64                 | 15.6%    | 41.6              | 2.3              | 4.3%               | 1.7%           | 0.0%             | 0.0%             | 0.0%              |
| DwtDet       | RivaGAN            | -            | parallel | -    | 64                 | 15.6%    | 41.5              | 2.4              | 4.2%               | 2.4%           | 0.0%             | 0.0%             | 0.0%              |
| DwtDet       | RivaGAN            | -            | series   | 0.5  | 64                 | 34.5%    | 39.7              | 2.1              | 8.4%               | 3.3%           | 0.0%             | 0.0%             | 0.0%              |
| DwtDet       | RivaGAN            | -            | series   | -    | 64                 | 43.9%    | 36.1              | 2.6              | 10.4%              | 5.1%           | 0.0%             | 0.0%             | 0.0%              |
| DwtDet       | RoSteALS           | -            | parallel | 0.5  | 132                | 2.5%     | 36.3              | 3.4              | 0.9%               | 0.3%           | 0.0%             | 0.0%             | 0.0%              |
| DwtDet       | RoSteALS           | -            | parallel | -    | 132                | 2.5%     | 36.2              | 3.4              | 0.7%               | 0.3%           | 0.0%             | 0.0%             | 0.0%              |
| DwtDet       | RoSteALS           | -            | series   | 0.5  | 132                | 7.0%     | 34.8              | 3.3              | 1.7%               | 0.7%           | 0.0%             | 0.0%             | 0.0%              |
| DwtDet       | RoSteALS           | -            | series   | -    | 132                | 35.1%    | 30.4              | 3.5              | 8.3%               | 4.8%           | 0.0%             | 0.0%             | 0.0%              |
| DwtDet       | SSL (42dB,30bits)  | -            | series   | 0.5  | 62                 | 39.1%    | 40.2              | 2.1              | 9.4%               | 4.8%           | 0.0%             | 0.0%             | 0.0%              |
| DwtDet       | SSL (42dB,30bits)  | -            | series   | -    | 62                 | 49.5%    | 36.5              | 2.9              | 11.9%              | 6.5%           | 0.1%             | 0.0%             | 0.0%              |
| DwtDet       | Trustmark B (0.95) | -            | parallel | 0.5  | 132                | 2.2%     | 41.8              | 2.6              | 0.7%               | 0.2%           | 0.0%             | 0.0%             | 0.0%              |
| DwtDet       | Trustmark B (0.95) | -            | parallel | -    | 132                | 2.2%     | 41.7              | 2.6              | 0.6%               | 0.2%           | 0.0%             | 0.0%             | 0.0%              |
| DwtDet       | Trustmark B (0.95) | -            | series   | 0.5  | 132                | 20.1%    | 39.7              | 2.4              | 4.4%               | 2.6%           | 0.0%             | 0.0%             | 0.0%              |
| DwtDet       | Trustmark B (0.95) | -            | series   | -    | 132                | 49.7%    | 36.2              | 2.8              | 12.9%              | 5.7%           | 0.0%             | 0.0%             | 0.0%              |
| DwtDet       | Trustmark Q (0.95) | -            | parallel | 0.5  | 132                | 1.8%     | 42.1              | 2.7              | 0.6%               | 0.2%           | 0.0%             | 0.0%             | 0.0%              |
| DwtDet       | Trustmark Q (0.95) | -            | parallel | -    | 132                | 1.8%     | 42.1              | 2.8              | 0.5%               | 0.3%           | 0.0%             | 0.0%             | 0.0%              |
| DwtDet       | Trustmark Q (0.95) | -            | series   | 0.5  | 132                | 15.9%    | 40.3              | 2.5              | 3.6%               | 1.4%           | 0.0%             | 0.0%             | 0.0%              |
| DwtDet       | Trustmark Q (0.95) | -            | series   | -    | 132                | 49.5%    | 36.6              | 3.0              | 13.2%              | 5.6%           | 0.0%             | 0.0%             | 0.0%              |
| DwtDetSvd    | DwtDet             | -            | series   | 0.5  | 64                 | 41.7%    | 39.8              | 2.5              | 11.5%              | 4.7%           | 0.0%             | 0.0%             | 0.1%              |
| DwtDetSvd    | DwtDet             | -            | series   | -    | 64                 | 46.4%    | 39.1              | 1.9              | 11.8%              | 4.8%           | 0.0%             | 0.0%             | 0.0%              |
| DwtDetSvd    | DwtDetSvd          | -            | parallel | 0.5  | 64                 | 0.0%     | 38.8              | 4.3              | 0.0%               | 0.0%           | 0.0%             | 0.0%             | 0.0%              |
| DwtDetSvd    | DwtDetSvd          | -            | parallel | -    | 64                 | 0.0%     | 38.8              | 4.3              | 0.0%               | 0.0%           | 0.0%             | 0.0%             | 0.0%              |
| DwtDetSvd    | DwtDetSvd          | -            | series   | 0.5  | 64                 | 0.0%     | 41.5              | 2.4              | 0.0%               | 0.0%           | 0.0%             | 0.0%             | 0.0%              |
| DwtDetSvd    | DwtDetSvd          | -            | series   | -    | 64                 | 0.0%     | 41.5              | 2.3              | 0.0%               | 0.0%           | 0.0%             | 0.0%             | 0.0%              |
| DwtDetSvd    | HiDDeN             | -            | parallel | 0.5  | 80                 | 0.1%     | 37.1              | 3.8              | 0.0%               | 0.0%           | 0.0%             | 0.0%             | 0.0%              |
| DwtDetSvd    | HiDDeN             | -            | parallel | -    | 80                 | 0.1%     | 37.0              | 4.0              | 0.0%               | 0.0%           | 0.0%             | 0.0%             | 0.0%              |
| DwtDetSvd    | HiDDeN             | -            | series   | 0.5  | 80                 | 2.3%     | 35.4              | 3.5              | 0.5%               | 0.2%           | 0.0%             | 0.0%             | 0.0%              |
| DwtDetSvd    | HiDDeN             | -            | series   | -    | 80                 | 11.6%    | 31.8              | 3.9              | 2.6%               | 1.7%           | 0.0%             | 0.0%             | 0.0%              |
| DwtDetSvd    | -                  | -            | -        | -    | 32                 | 85.0%    | 38.3              | 3.9              | 20.3%              | 15.5%          | 0.3%             | 0.2%             | 0.1%              |
| DwtDetSvd    | RivaGAN            | LC[64,36,12] | parallel | -0.2 | 36                 | 55.5%    | 41.3              | 2.3              | 13.8%              | 9.7%           | 0.1%             | 0.0%             | 0.0%              |
| DwtDetSvd    | RivaGAN            | LC[64,36,12] | parallel | -0.1 | 36                 | 55.5%    | 41.3              | 2.3              | 12.9%              | 10.0%          | 0.2%             | 0.3%             | 0.0%              |
| DwtDetSvd    | RivaGAN            | LC[64,36,12] | parallel | 0    | 36                 | 55.5%    | 41.3              | 2.3              | 13.6%              | 9.0%           | 0.0%             | 0.1%             | 0.0%              |
| DwtDetSvd    | RivaGAN            | LC[64,36,12] | parallel | 0.1  | 36                 | 55.5%    | 41.3              | 2.3              | 14.5%              | 9.4%           | 0.1%             | 0.0%             | 0.1%              |
| DwtDetSvd    | RivaGAN            | LC[64,36,12] | parallel | 0.2  | 36                 | 55.5%    | 41.3              | 2.3              | 14.5%              | 10.6%          | 0.1%             | 0.0%             | 0.0%              |
| DwtDetSvd    | RivaGAN            | LC[64,36,12] | parallel | 0.3  | 36                 | 55.5%    | 41.3              | 2.3              | 13.8%              | 10.9%          | 0.1%             | 0.0%             | 0.1%              |
| DwtDetSvd    | RivaGAN            | LC[64,36,12] | parallel | 0.4  | 36                 | 55.5%    | 41.3              | 2.3              | 13.2%              | 9.0%           | 0.0%             | 0.1%             | 0.0%              |
| DwtDetSvd    | RivaGAN            | LC[64,36,12] | parallel | 0.5  | 36                 | 55.4%    | 41.4              | 2.2              | 14.7%              | 9.8%           | 0.1%             | 0.1%             | 0.0%              |
| DwtDetSvd    | RivaGAN            | LC[64,36,12] | parallel | 0.6  | 36                 | 55.3%    | 41.5              | 2.2              | 13.9%              | 9.4%           | 0.1%             | 0.2%             | 0.2%              |
| DwtDetSvd    | RivaGAN            | LC[64,36,12] | parallel | 0.7  | 36                 | 55.2%    | 41.5              | 2.0              | 13.3%              | 8.8%           | 0.3%             | 0.1%             | 0.0%              |
| DwtDetSvd    | RivaGAN            | LC[64,36,12] | parallel | 0.8  | 36                 | 54.7%    | 41.7              | 1.9              | 14.1%              | 10.2%          | 0.1%             | 0.1%             | 0.1%              |
| DwtDetSvd    | RivaGAN            | LC[64,36,12] | parallel | 0.9  | 36                 | 54.0%    | 41.9              | 1.8              | 12.9%              | 9.9%           | 0.0%             | 0.0%             | 0.0%              |
| DwtDetSvd    | RivaGAN            | LC[64,36,12] | parallel | 1    | 36                 | 53.0%    | 42.1              | 1.8              | 12.3%              | 8.9%           | 0.2%             | 0.1%             | 0.1%              |
| DwtDetSvd    | RivaGAN            | LC[64,36,12] | parallel | 1.1  | 36                 | 51.8%    | 42.3              | 1.7              | 13.0%              | 9.2%           | 0.0%             | 0.0%             | 0.1%              |
| DwtDetSvd    | RivaGAN            | LC[64,36,12] | parallel | 1.2  | 36                 | 50.2%    | 42.6              | 1.7              | 12.5%              | 8.9%           | 0.0%             | 0.0%             | 0.0%              |
| DwtDetSvd    | RivaGAN            | LC[64,36,12] | parallel | -    | 36                 | 55.5%    | 41.3              | 2.3              | 14.1%              | 10.0%          | 0.1%             | 0.4%             | 0.0%              |
| DwtDetSvd    | RivaGAN            | LC[64,36,12] | series   | -0.2 | 36                 | 53.4%    | 37.3              | 3.3              | 13.1%              | 10.5%          | 0.2%             | 0.2%             | 0.1%              |
| DwtDetSvd    | RivaGAN            | LC[64,36,12] | series   | -0.1 | 36                 | 54.0%    | 37.4              | 3.3              | 13.5%              | 10.2%          | 0.1%             | 0.2%             | 0.1%              |
| DwtDetSvd    | RivaGAN            | LC[64,36,12] | series   | 0    | 36                 | 54.6%    | 37.7              | 3.2              | 12.7%              | 9.5%           | 0.4%             | 0.1%             | 0.0%              |
| DwtDetSvd    | RivaGAN            | LC[64,36,12] | series   | 0.1  | 36                 | 54.3%    | 38.1              | 3.0              | 14.7%              | 9.7%           | 0.0%             | 0.1%             | 0.2%              |
| DwtDetSvd    | RivaGAN            | LC[64,36,12] | series   | 0.2  | 36                 | 53.3%    | 38.5              | 2.8              | 13.1%              | 9.3%           | 0.1%             | 0.2%             | 0.0%              |
| DwtDetSvd    | RivaGAN            | LC[64,36,12] | series   | 0.3  | 36                 | 54.7%    | 39.0              | 2.5              | 14.0%              | 10.0%          | 0.0%             | 0.1%             | 0.1%              |
| DwtDetSvd    | RivaGAN            | LC[64,36,12] | series   | 0.4  | 36                 | 54.2%    | 39.3              | 2.3              | 13.5%              | 8.8%           | 0.2%             | 0.0%             | 0.0%              |
| DwtDetSvd    | RivaGAN            | LC[64,36,12] | series   | 0.5  | 36                 | 54.0%    | 39.7              | 2.1              | 14.1%              | 9.5%           | 0.1%             | 0.1%             | 0.2%              |
| DwtDetSvd    | RivaGAN            | LC[64,36,12] | series   | 0.6  | 36                 | 53.4%    | 40.0              | 2.0              | 12.7%              | 9.3%           | 0.1%             | 0.0%             | 0.1%              |
| DwtDetSvd    | RivaGAN            | LC[64,36,12] | series   | 0.7  | 36                 | 52.6%    | 40.3              | 1.8              | 12.5%              | 10.4%          | 0.1%             | 0.1%             | 0.0%              |
| DwtDetSvd    | RivaGAN            | LC[64,36,12] | series   | 0.8  | 36                 | 52.1%    | 40.6              | 1.7              | 13.2%              | 9.1%           | 0.2%             | 0.0%             | 0.0%              |
| DwtDetSvd    | RivaGAN            | LC[64,36,12] | series   | 0.9  | 36                 | 51.2%    | 41.0              | 1.8              | 13.1%              | 8.4%           | 0.0%             | 0.0%             | 0.2%              |
| DwtDetSvd    | RivaGAN            | LC[64,36,12] | series   | 1    | 36                 | 49.4%    | 41.3              | 1.8              | 12.0%              | 9.2%           | 0.0%             | 0.0%             | 0.0%              |
| DwtDetSvd    | RivaGAN            | LC[64,36,12] | series   | 1.1  | 36                 | 48.2%    | 41.6              | 1.8              | 12.1%              | 8.7%           | 0.1%             | 0.0%             | 0.1%              |
| DwtDetSvd    | RivaGAN            | LC[64,36,12] | series   | 1.2  | 36                 | 47.0%    | 42.0              | 1.8              | 12.0%              | 8.2%           | 0.1%             | 0.1%             | 0.0%              |
| DwtDetSvd    | RivaGAN            | LC[64,36,12] | series   | -    | 36                 | 53.4%    | 36.1              | 2.6              | 14.6%              | 10.4%          | 0.0%             | 0.2%             | 0.0%              |
| DwtDetSvd    | RivaGAN            | -            | parallel | 0.5  | 64                 | 34.5%    | 41.4              | 2.2              | 9.3%               | 4.9%           | 0.0%             | 0.0%             | 0.0%              |
| DwtDetSvd    | RivaGAN            | -            | parallel | -    | 64                 | 34.5%    | 41.3              | 2.3              | 8.8%               | 5.0%           | 0.0%             | 0.0%             | 0.0%              |
| DwtDetSvd    | RivaGAN            | -            | series   | 0.5  | 64                 | 32.8%    | 39.7              | 2.1              | 8.9%               | 4.7%           | 0.0%             | 0.1%             | 0.0%              |
| DwtDetSvd    | RivaGAN            | -            | series   | -    | 64                 | 36.4%    | 36.1              | 2.6              | 9.8%               | 6.9%           | 0.0%             | 0.0%             | 0.0%              |
| DwtDetSvd    | RoSteALS           | -            | parallel | 0.5  | 132                | 5.2%     | 36.3              | 3.4              | 1.1%               | 0.8%           | 0.0%             | 0.0%             | 0.0%              |
| DwtDetSvd    | RoSteALS           | -            | parallel | -    | 132                | 5.2%     | 36.2              | 3.4              | 1.8%               | 0.6%           | 0.0%             | 0.0%             | 0.0%              |
| DwtDetSvd    | RoSteALS           | -            | series   | 0.5  | 132                | 2.0%     | 34.8              | 3.4              | 0.5%               | 0.1%           | 0.0%             | 0.0%             | 0.0%              |
| DwtDetSvd    | RoSteALS           | -            | series   | -    | 132                | 3.0%     | 30.4              | 3.5              | 1.0%               | 0.4%           | 0.0%             | 0.0%             | 0.0%              |
| DwtDetSvd    | SSL (42dB,30bits)  | -            | series   | 0.5  | 62                 | 62.1%    | 40.1              | 2.1              | 15.2%              | 8.8%           | 0.0%             | 0.0%             | 0.1%              |
| DwtDetSvd    | SSL (42dB,30bits)  | -            | series   | -    | 62                 | 80.2%    | 36.4              | 2.8              | 19.7%              | 14.0%          | 0.0%             | 0.1%             | 0.2%              |
| DwtDetSvd    | Trustmark B (0.95) | -            | parallel | 0.5  | 132                | 4.9%     | 41.5              | 2.5              | 1.1%               | 0.9%           | 0.0%             | 0.0%             | 0.0%              |
| DwtDetSvd    | Trustmark B (0.95) | -            | parallel | -    | 132                | 5.0%     | 41.5              | 2.6              | 1.5%               | 0.7%           | 0.0%             | 0.0%             | 0.0%              |

| First method | Second method      | ECC           | Ensemble | Clip | Capacity<br>(bits) | Accuracy | Mean<br>PSNR [dB] | Std<br>PSNR [dB] | Robust.<br>RivaGAN | Robust.<br>SSL | Robust.<br>TmLow | Robust.<br>TmMed | Robust.<br>TmHigh |
|--------------|--------------------|---------------|----------|------|--------------------|----------|-------------------|------------------|--------------------|----------------|------------------|------------------|-------------------|
| DwtDctSvd    | Trustmark B (0.95) | -             | series   | 0.5  | 132                | 26.9%    | 39.7              | 2.5              | 6.7%               | 3.7%           | 0.0%             | 0.0%             | 0.0%              |
| DwtDctSvd    | Trustmark B (0.95) | -             | series   | -    | 132                | 79.5%    | 36.0              | 2.8              | 19.4%              | 13.5%          | 0.2%             | 0.2%             | 0.0%              |
| DwtDctSvd    | Trustmark Q (0.95) | -             | parallel | 0.5  | 132                | 4.2%     | 41.9              | 2.7              | 1.2%               | 1.1%           | 0.0%             | 0.0%             | 0.0%              |
| DwtDctSvd    | Trustmark Q (0.95) | -             | parallel | -    | 132                | 4.3%     | 41.9              | 2.8              | 1.4%               | 0.7%           | 0.1%             | 0.0%             | 0.0%              |
| DwtDctSvd    | Trustmark Q (0.95) | -             | series   | 0.5  | 132                | 22.9%    | 40.3              | 2.6              | 5.8%               | 3.2%           | 0.0%             | 0.1%             | 0.0%              |
| DwtDctSvd    | Trustmark Q (0.95) | -             | series   | -    | 132                | 76.9%    | 36.5              | 3.0              | 19.3%              | 11.9%          | 0.1%             | 0.0%             | 0.1%              |
| HiDDeN       | DwtDct             | -             | series   | 0.5  | 80                 | 1.0%     | 35.5              | 3.5              | 0.1%               | 0.1%           | 0.0%             | 0.0%             | 0.0%              |
| HiDDeN       | DwtDct             | -             | series   | -    | 80                 | 8.6%     | 31.5              | 3.9              | 2.8%               | 1.0%           | 0.0%             | 0.0%             | 0.0%              |
| HiDDeN       | DwtDctSvd          | -             | series   | 0.5  | 80                 | 1.5%     | 35.5              | 3.5              | 0.3%               | 0.1%           | 0.0%             | 0.0%             | 0.0%              |
| HiDDeN       | DwtDctSvd          | -             | series   | -    | 80                 | 13.2%    | 31.5              | 3.9              | 3.2%               | 1.5%           | 0.0%             | 0.0%             | 0.0%              |
| HiDDeN       | HiDDeN             | -             | parallel | 0.5  | 96                 | 0.0%     | 33.2              | 4.8              | 0.0%               | 0.0%           | 0.0%             | 0.0%             | 0.0%              |
| HiDDeN       | HiDDeN             | -             | parallel | -    | 96                 | 0.0%     | 33.2              | 4.8              | 0.0%               | 0.0%           | 0.0%             | 0.0%             | 0.0%              |
| HiDDeN       | HiDDeN             | -             | series   | 0.5  | 96                 | 0.0%     | 32.6              | 4.5              | 0.0%               | 0.0%           | 0.0%             | 0.0%             | 0.0%              |
| HiDDeN       | HiDDeN             | -             | series   | -    | 96                 | 0.0%     | 30.8              | 4.1              | 0.0%               | 0.0%           | 0.0%             | 0.0%             | 0.0%              |
| HiDDeN       | -                  | -             | -        | -    | 48                 | 15.0%    | 32.7              | 4.5              | 5.3%               | 1.9%           | 0.1%             | 0.0%             | 0.1%              |
| HiDDeN       | RivaGAN            | -             | series   | 0.5  | 80                 | 0.3%     | 36.7              | 2.3              | 0.0%               | 0.0%           | 0.0%             | 0.0%             | 0.0%              |
| HiDDeN       | RivaGAN            | -             | series   | -    | 80                 | 9.4%     | 31.8              | 3.8              | 2.4%               | 1.2%           | 0.0%             | 0.0%             | 0.1%              |
| HiDDeN       | RoSteALS           | LC[148,49,34] | series   | -0.2 | 49                 | 81.6%    | 30.2              | 3.8              | 38.8%              | 16.5%          | 0.2%             | 0.1%             | 0.2%              |
| HiDDeN       | RoSteALS           | LC[148,49,34] | series   | -0.1 | 49                 | 80.5%    | 30.4              | 3.8              | 40.1%              | 18.1%          | 0.2%             | 0.2%             | 0.0%              |
| HiDDeN       | RoSteALS           | LC[148,49,34] | series   | 0    | 49                 | 79.2%    | 30.7              | 3.8              | 35.5%              | 14.3%          | 0.1%             | 0.1%             | 0.1%              |
| HiDDeN       | RoSteALS           | LC[148,49,34] | series   | 0.1  | 49                 | 78.3%    | 31.0              | 3.8              | 37.9%              | 15.1%          | 0.0%             | 0.0%             | 0.0%              |
| HiDDeN       | RoSteALS           | LC[148,49,34] | series   | 0.2  | 49                 | 77.6%    | 31.2              | 3.8              | 35.9%              | 15.1%          | 0.0%             | 0.2%             | 0.2%              |
| HiDDeN       | RoSteALS           | LC[148,49,34] | series   | 0.3  | 49                 | 75.6%    | 31.5              | 3.8              | 35.0%              | 14.0%          | 0.0%             | 0.1%             | 0.1%              |
| HiDDeN       | RoSteALS           | LC[148,49,34] | series   | 0.4  | 49                 | 72.3%    | 31.7              | 3.8              | 34.1%              | 14.3%          | 0.1%             | 0.1%             | 0.1%              |
| HiDDeN       | RoSteALS           | LC[148,49,34] | series   | 0.5  | 49                 | 70.6%    | 32.0              | 3.8              | 33.6%              | 12.8%          | 0.1%             | 0.1%             | 0.0%              |
| HiDDeN       | RoSteALS           | LC[148,49,34] | series   | 0.6  | 49                 | 68.5%    | 32.3              | 3.8              | 31.3%              | 12.3%          | 0.0%             | 0.0%             | 0.0%              |
| HiDDeN       | RoSteALS           | LC[148,49,34] | series   | 0.7  | 49                 | 66.7%    | 32.5              | 3.8              | 30.3%              | 12.8%          | 0.1%             | 0.2%             | 0.1%              |
| HiDDeN       | RoSteALS           | LC[148,49,34] | series   | 0.8  | 49                 | 65.0%    | 32.8              | 3.9              | 29.2%              | 10.7%          | 0.1%             | 0.2%             | 0.2%              |
| HiDDeN       | RoSteALS           | LC[148,49,34] | series   | 0.9  | 49                 | 62.9%    | 33.0              | 4.0              | 29.1%              | 11.9%          | 0.2%             | 0.1%             | 0.0%              |
| HiDDeN       | RoSteALS           | LC[148,49,34] | series   | 1    | 49                 | 61.0%    | 33.3              | 4.0              | 27.9%              | 10.7%          | 0.0%             | 0.0%             | 0.0%              |
| HiDDeN       | RoSteALS           | LC[148,49,34] | series   | 1.1  | 49                 | 58.8%    | 33.5              | 4.1              | 27.9%              | 10.8%          | 0.1%             | 0.0%             | 0.0%              |
| HiDDeN       | RoSteALS           | LC[148,49,34] | series   | 1.2  | 49                 | 56.9%    | 33.8              | 4.2              | 26.7%              | 9.7%           | 0.0%             | 0.0%             | 0.1%              |
| HiDDeN       | RoSteALS           | LC[148,49,34] | series   | -    | 49                 | 85.6%    | 28.8              | 3.8              | 40.8%              | 16.4%          | 0.1%             | 0.3%             | 0.3%              |
| HiDDeN       | RoSteALS           | -             | series   | 0.5  | 148                | 0.0%     | 32.0              | 3.8              | 0.0%               | 0.0%           | 0.0%             | 0.0%             | 0.0%              |
| HiDDeN       | RoSteALS           | -             | series   | -    | 148                | 1.8%     | 28.8              | 3.8              | 1.0%               | 0.1%           | 0.0%             | 0.0%             | 0.0%              |
| HiDDeN       | SSL (42dB,30bits)  | -             | series   | 0.5  | 78                 | 0.1%     | 37.3              | 2.3              | 0.0%               | 0.0%           | 0.0%             | 0.0%             | 0.0%              |
| HiDDeN       | SSL (42dB,30bits)  | -             | series   | -    | 78                 | 14.4%    | 32.0              | 3.9              | 4.7%               | 1.4%           | 0.1%             | 0.0%             | 0.0%              |
| HiDDeN       | Trustmark B (0.95) | -             | parallel | 0.5  | 148                | 0.0%     | 37.9              | 3.5              | 0.0%               | 0.0%           | 0.0%             | 0.0%             | 0.0%              |
| HiDDeN       | Trustmark B (0.95) | -             | parallel | -    | 148                | 0.0%     | 37.7              | 3.9              | 0.0%               | 0.0%           | 0.0%             | 0.0%             | 0.0%              |
| HiDDeN       | Trustmark B (0.95) | -             | series   | 0.5  | 148                | 0.1%     | 36.9              | 3.0              | 0.0%               | 0.0%           | 0.0%             | 0.0%             | 0.0%              |
| HiDDeN       | Trustmark B (0.95) | -             | series   | -    | 148                | 12.5%    | 31.9              | 4.0              | 4.2%               | 1.7%           | 0.0%             | 0.0%             | 0.0%              |
| HiDDeN       | Trustmark Q (0.95) | -             | parallel | 0.5  | 148                | 0.0%     | 38.2              | 3.5              | 0.0%               | 0.0%           | 0.0%             | 0.0%             | 0.0%              |
| HiDDeN       | Trustmark Q (0.95) | -             | parallel | -    | 148                | 0.0%     | 37.9              | 4.0              | 0.0%               | 0.0%           | 0.0%             | 0.0%             | 0.0%              |
| HiDDeN       | Trustmark Q (0.95) | -             | series   | 0.5  | 148                | 0.0%     | 37.5              | 3.1              | 0.0%               | 0.0%           | 0.0%             | 0.0%             | 0.0%              |
| HiDDeN       | Trustmark Q (0.95) | -             | series   | -    | 148                | 10.4%    | 32.1              | 4.2              | 3.2%               | 1.3%           | 0.1%             | 0.0%             | 0.0%              |
| RivaGAN      | DwtDct             | -             | series   | 0.5  | 64                 | 38.5%    | 39.7              | 2.1              | 10.8%              | 4.1%           | 0.0%             | 0.0%             | 0.1%              |
| RivaGAN      | DwtDct             | -             | series   | -    | 64                 | 43.3%    | 36.0              | 2.6              | 11.0%              | 5.8%           | 0.1%             | 0.0%             | 0.0%              |
| RivaGAN      | DwtDctSvd          | LC[64,36,12]  | series   | -0.2 | 36                 | 85.0%    | 37.3              | 3.4              | 20.5%              | 15.3%          | 0.4%             | 0.2%             | 0.2%              |
| RivaGAN      | DwtDctSvd          | LC[64,36,12]  | series   | -0.1 | 36                 | 84.5%    | 37.5              | 3.4              | 19.9%              | 17.6%          | 0.1%             | 0.2%             | 0.2%              |
| RivaGAN      | DwtDctSvd          | LC[64,36,12]  | series   | 0    | 36                 | 84.2%    | 37.8              | 3.3              | 19.6%              | 16.1%          | 0.3%             | 0.1%             | 0.0%              |
| RivaGAN      | DwtDctSvd          | LC[64,36,12]  | series   | 0.1  | 36                 | 82.8%    | 38.2              | 3.0              | 19.6%              | 15.2%          | 0.2%             | 0.2%             | 0.2%              |
| RivaGAN      | DwtDctSvd          | LC[64,36,12]  | series   | 0.2  | 36                 | 81.5%    | 38.5              | 2.7              | 20.1%              | 15.0%          | 0.1%             | 0.1%             | 0.1%              |
| RivaGAN      | DwtDctSvd          | LC[64,36,12]  | series   | 0.3  | 36                 | 78.7%    | 39.0              | 2.5              | 21.2%              | 15.4%          | 0.2%             | 0.4%             | 0.1%              |
| RivaGAN      | DwtDctSvd          | LC[64,36,12]  | series   | 0.4  | 36                 | 77.1%    | 39.3              | 2.3              | 18.6%              | 13.5%          | 0.2%             | 0.2%             | 0.2%              |
| RivaGAN      | DwtDctSvd          | LC[64,36,12]  | series   | 0.5  | 36                 | 74.8%    | 39.6              | 2.1              | 18.7%              | 13.6%          | 0.1%             | 0.1%             | 0.1%              |
| RivaGAN      | DwtDctSvd          | LC[64,36,12]  | series   | 0.6  | 36                 | 72.7%    | 39.9              | 1.9              | 18.5%              | 13.9%          | 0.3%             | 0.1%             | 0.1%              |
| RivaGAN      | DwtDctSvd          | LC[64,36,12]  | series   | 0.7  | 36                 | 70.1%    | 40.2              | 1.7              | 16.2%              | 11.3%          | 0.3%             | 0.2%             | 0.2%              |
| RivaGAN      | DwtDctSvd          | LC[64,36,12]  | series   | 0.8  | 36                 | 67.1%    | 40.6              | 1.8              | 16.5%              | 12.5%          | 0.1%             | 0.1%             | 0.0%              |
| RivaGAN      | DwtDctSvd          | LC[64,36,12]  | series   | 0.9  | 36                 | 64.0%    | 40.9              | 1.8              | 15.1%              | 10.6%          | 0.1%             | 0.1%             | 0.2%              |
| RivaGAN      | DwtDctSvd          | LC[64,36,12]  | series   | 1    | 36                 | 61.3%    | 41.3              | 1.8              | 15.4%              | 11.0%          | 0.1%             | 0.2%             | 0.0%              |
| RivaGAN      | DwtDctSvd          | LC[64,36,12]  | series   | 1.1  | 36                 | 58.7%    | 41.6              | 1.9              | 16.3%              | 10.1%          | 0.1%             | 0.2%             | 0.1%              |
| RivaGAN      | DwtDctSvd          | LC[64,36,12]  | series   | 1.2  | 36                 | 55.9%    | 42.0              | 2.0              | 13.1%              | 10.5%          | 0.1%             | 0.1%             | 0.1%              |
| RivaGAN      | DwtDctSvd          | LC[64,36,12]  | series   | -    | 36                 | 86.9%    | 36.0              | 2.6              | 21.2%              | 16.2%          | 0.2%             | 0.1%             | 0.0%              |
| RivaGAN      | DwtDctSvd          | -             | series   | 0.5  | 64                 | 57.3%    | 39.6              | 2.1              | 13.9%              | 8.8%           | 0.0%             | 0.0%             | 0.0%              |
| RivaGAN      | DwtDctSvd          | -             | series   | -    | 64                 | 69.9%    | 36.0              | 2.6              | 17.2%              | 11.8%          | 0.1%             | 0.1%             | 0.0%              |
| RivaGAN      | HiDDeN             | -             | parallel | 0.5  | 80                 | 0.2%     | 37.9              | 3.1              | 0.0%               | 0.0%           | 0.0%             | 0.0%             | 0.0%              |
| RivaGAN      | HiDDeN             | -             | parallel | -    | 80                 | 0.2%     | 37.6              | 3.7              | 0.1%               | 0.0%           | 0.0%             | 0.0%             | 0.0%              |
| RivaGAN      | HiDDeN             | -             | series   | 0.5  | 80                 | 0.5%     | 36.7              | 2.3              | 0.1%               | 0.1%           | 0.0%             | 0.0%             | 0.0%              |
| RivaGAN      | HiDDeN             | -             | series   | -    | 80                 | 11.9%    | 31.8              | 3.8              | 3.7%               | 1.5%           | 0.0%             | 0.0%             | 0.0%              |
| RivaGAN      | -                  | -             | -        | -    | 32                 | 75.8%    | 40.8              | 0.6              | 72.9%              | 29.3%          | 28.7%            | 27.3%            | 24.8%             |
| RivaGAN      | RivaGAN            | -             | parallel | 0.5  | 64                 | 0.0%     | 42.6              | 0.9              | 0.0%               | 0.0%           | 0.0%             | 0.0%             | 0.0%              |
| RivaGAN      | RivaGAN            | -             | parallel | -    | 64                 | 0.0%     | 42.6              | 0.9              | 0.0%               | 0.0%           | 0.0%             | 0.0%             | 0.0%              |
| RivaGAN      | RivaGAN            | -             | series   | 0.5  | 64                 | 0.0%     | 40.7              | 0.7              | 0.0%               | 0.0%           | 0.0%             | 0.0%             | 0.0%              |
| RivaGAN      | RivaGAN            | -             | series   | -    | 64                 | 0.0%     | 37.8              | 1.2              | 0.0%               | 0.0%           | 0.0%             | 0.0%             | 0.0%              |
| RivaGAN      | RoSteALS           | LC[131,32,37] | parallel | -0.2 | 32                 | 97.4%    | 36.4              | 3.0              | 51.6%              | 28.4%          | 0.2%             | 0.0%             | 0.2%              |
| RivaGAN      | RoSteALS           | LC[131,32,37] | parallel | -0.1 | 32                 | 97.4%    | 36.4              | 3.0              | 48.9%              | 28.7%          | 0.4%             | 0.4%             | 0.4%              |
| RivaGAN      | RoSteALS           | LC[131,32,37] | parallel | 0    | 32                 | 97.4%    | 36.4              | 3.0              | 52.3%              | 27.7%          | 0.4%             | 0.4%             | 0.4%              |
| RivaGAN      | RoSteALS           | LC[131,32,37] | parallel | 0.1  | 32                 | 97.4%    | 36.4              | 3.0              | 48.3%              | 29.3%          | 0.3%             | 0.7%             | 0.2%              |
| RivaGAN      | RoSteALS           | LC[131,32,37] | parallel | 0.2  | 32                 | 97.4%    | 36.4              | 3.0              | 48.2%              | 27.8%          | 0.3%             | 0.3%             | 0.4%              |
| RivaGAN      | RoSteALS           | LC[131,32,37] | parallel | 0.3  | 32                 | 97.4%    | 36.4              | 3.0              | 51.4%              | 29.2%          | 0.3%             | 0.2%             | 0.3%              |
| RivaGAN      | RoSteALS           | LC[131,32,37] | parallel | 0.4  | 32                 | 97.0%    | 36.5              | 2.9              | 49.0%              | 28.3%          | 0.6%             | 0.2%             | 0.1%              |
| RivaGAN      | RoSteALS           | LC[131,32,37] | parallel | 0.5  | 32                 | 94.9%    | 36.8              | 2.5              | 49.1%              | 29.0%          | 0.1%             | 0.5%             | 0.2%              |
| RivaGAN      | RoSteALS           | LC[131,32,37] | parallel | 0.6  | 32                 | 90.7%    | 37.3              | 2.0              | 46.8%              | 25.7%          | 0.5%             | 0.2%             | 0.3%              |
| RivaGAN      | RoSteALS           | LC[131,32,37] | parallel | 0.7  | 32                 | 85.0%    | 38.1              | 1.5              | 42.9%              | 22.5%          | 0.3%             | 0.2%             | 0.2%              |
| RivaGAN      | RoSteALS           | LC[131,32,37] | parallel | 0.8  | 32                 | 79.8%    | 39.0              | 1.1              | 40.6%              | 21.9%          | 0.4%             | 0.3%             | 0.1%              |
| RivaGAN      | RoSteALS           | LC[131,32,37] | parallel | 0.9  | 32                 | 74.5%    | 39.9              | 0.9              | 37.2%              | 20.0%          | 0.1%             | 0.0%             | 0.2%              |

| First method | Second method      | ECC            | Ensemble | Clip | Capacity<br>(bits) | Accuracy | Mean<br>PSNR [dB] | Std<br>PSNR [dB] | Robust.<br>RivaGAN | Robust.<br>SSL | Robust.<br>TmLow | Robust.<br>TmMed | Robust.<br>TmHigh |
|--------------|--------------------|----------------|----------|------|--------------------|----------|-------------------|------------------|--------------------|----------------|------------------|------------------|-------------------|
| RivaGAN      | RoSteALS           | LC[131,32,37]  | parallel | 1    | 32                 | 67.2%    | 40.8              | 0.7              | 32.4%              | 19.4%          | 0.1%             | 0.3%             | 0.2%              |
| RivaGAN      | RoSteALS           | LC[131,32,37]  | parallel | 1.1  | 32                 | 59.6%    | 41.8              | 0.8              | 30.2%              | 16.8%          | 0.0%             | 0.1%             | 0.1%              |
| RivaGAN      | RoSteALS           | LC[131,32,37]  | parallel | 1.2  | 32                 | 53.1%    | 42.7              | 1.0              | 26.4%              | 15.4%          | 0.3%             | 0.1%             | 0.0%              |
| RivaGAN      | RoSteALS           | LC[131,32,37]  | parallel | -    | 32                 | 97.4%    | 36.4              | 3.0              | 48.7%              | 29.3%          | 0.2%             | 0.3%             | 0.5%              |
| RivaGAN      | RoSteALS           | LC[131,32,37]  | series   | -0.2 | 32                 | 99.5%    | 31.0              | 3.4              | 51.1%              | 31.0%          | 0.6%             | 0.5%             | 0.8%              |
| RivaGAN      | RoSteALS           | LC[131,32,37]  | series   | -0.1 | 32                 | 99.5%    | 31.0              | 3.5              | 51.5%              | 31.3%          | 0.2%             | 0.4%             | 0.4%              |
| RivaGAN      | RoSteALS           | LC[131,32,37]  | series   | 0    | 32                 | 99.5%    | 31.3              | 3.6              | 50.9%              | 30.9%          | 0.4%             | 0.5%             | 0.2%              |
| RivaGAN      | RoSteALS           | LC[131,32,37]  | series   | 0.1  | 32                 | 99.1%    | 32.3              | 3.2              | 49.9%              | 32.1%          | 0.5%             | 0.5%             | 0.2%              |
| RivaGAN      | RoSteALS           | LC[131,32,37]  | series   | 0.2  | 32                 | 98.5%    | 33.2              | 2.9              | 51.2%              | 31.0%          | 0.2%             | 0.3%             | 0.4%              |
| RivaGAN      | RoSteALS           | LC[131,32,37]  | series   | 0.3  | 32                 | 96.9%    | 34.2              | 2.6              | 49.4%              | 28.7%          | 0.4%             | 0.4%             | 0.3%              |
| RivaGAN      | RoSteALS           | LC[131,32,37]  | series   | 0.4  | 32                 | 95.0%    | 35.1              | 2.2              | 47.2%              | 27.3%          | 0.4%             | 0.3%             | 0.3%              |
| RivaGAN      | RoSteALS           | LC[131,32,37]  | series   | 0.5  | 32                 | 91.7%    | 36.1              | 1.9              | 47.7%              | 25.4%          | 0.2%             | 0.3%             | 0.3%              |
| RivaGAN      | RoSteALS           | LC[131,32,37]  | series   | 0.6  | 32                 | 87.6%    | 37.0              | 1.6              | 44.7%              | 24.4%          | 0.3%             | 0.4%             | 0.3%              |
| RivaGAN      | RoSteALS           | LC[131,32,37]  | series   | 0.7  | 32                 | 82.9%    | 38.0              | 1.2              | 43.0%              | 22.9%          | 0.2%             | 0.2%             | 0.3%              |
| RivaGAN      | RoSteALS           | LC[131,32,37]  | series   | 0.8  | 32                 | 77.2%    | 38.9              | 1.0              | 38.4%              | 21.0%          | 0.3%             | 0.1%             | 0.3%              |
| RivaGAN      | RoSteALS           | LC[131,32,37]  | series   | 0.9  | 32                 | 71.7%    | 39.9              | 0.8              | 35.2%              | 19.3%          | 0.2%             | 0.2%             | 0.3%              |
| RivaGAN      | RoSteALS           | LC[131,32,37]  | series   | 1    | 32                 | 65.3%    | 40.8              | 0.7              | 32.5%              | 16.5%          | 0.2%             | 0.0%             | 0.1%              |
| RivaGAN      | RoSteALS           | LC[131,32,37]  | series   | 1.1  | 32                 | 58.1%    | 41.7              | 0.7              | 27.1%              | 16.0%          | 0.1%             | 0.2%             | 0.1%              |
| RivaGAN      | RoSteALS           | LC[131,32,37]  | series   | 1.2  | 32                 | 51.6%    | 42.7              | 0.9              | 24.8%              | 13.1%          | 0.1%             | 0.0%             | 0.1%              |
| RivaGAN      | RoSteALS           | LC[131,32,37]  | series   | -    | 32                 | 99.4%    | 30.9              | 3.3              | 51.4%              | 29.8%          | 0.4%             | 0.3%             | 0.6%              |
| RivaGAN      | RoSteALS           | -              | parallel | 0.5  | 132                | 4.3%     | 36.8              | 2.5              | 2.3%               | 0.7%           | 0.0%             | 0.0%             | 0.0%              |
| RivaGAN      | RoSteALS           | -              | parallel | -    | 132                | 4.3%     | 36.4              | 3.0              | 2.1%               | 0.9%           | 0.0%             | 0.0%             | 0.0%              |
| RivaGAN      | RoSteALS           | -              | series   | 0.5  | 132                | 5.9%     | 36.1              | 1.9              | 2.4%               | 0.7%           | 0.0%             | 0.0%             | 0.0%              |
| RivaGAN      | RoSteALS           | -              | series   | -    | 132                | 24.0%    | 30.9              | 3.3              | 10.7%              | 5.6%           | 0.0%             | 0.0%             | 0.0%              |
| RivaGAN      | SSL (42dB,30bits)  | -              | series   | 0.5  | 62                 | 63.7%    | 41.4              | 0.6              | 50.9%              | 20.7%          | 13.9%            | 11.8%            | 10.4%             |
| RivaGAN      | SSL (42dB,30bits)  | -              | series   | -    | 62                 | 69.9%    | 38.4              | 0.6              | 64.8%              | 24.7%          | 21.0%            | 19.1%            | 15.3%             |
| RivaGAN      | Trustmark B (0.95) | -              | parallel | 0.5  | 132                | 2.9%     | 42.8              | 1.2              | 4.3%               | 0.7%           | 1.0%             | 1.4%             | 0.8%              |
| RivaGAN      | Trustmark B (0.95) | -              | parallel | -    | 132                | 2.9%     | 42.8              | 1.2              | 4.3%               | 0.7%           | 1.0%             | 1.0%             | 1.1%              |
| RivaGAN      | Trustmark B (0.95) | -              | series   | 0.5  | 132                | 26.3%    | 40.9              | 1.1              | 28.4%              | 5.7%           | 9.8%             | 9.0%             | 8.1%              |
| RivaGAN      | Trustmark B (0.95) | -              | series   | -    | 132                | 68.0%    | 37.5              | 1.1              | 64.8%              | 18.9%          | 22.9%            | 21.4%            | 18.0%             |
| RivaGAN      | Trustmark Q (0.95) | -              | parallel | 0.5  | 132                | 3.5%     | 43.3              | 1.2              | 4.1%               | 0.6%           | 1.1%             | 0.8%             | 0.6%              |
| RivaGAN      | Trustmark Q (0.95) | -              | parallel | -    | 132                | 3.5%     | 43.3              | 1.2              | 4.2%               | 0.8%           | 0.7%             | 0.6%             | 0.4%              |
| RivaGAN      | Trustmark Q (0.95) | -              | series   | 0.5  | 132                | 21.6%    | 41.5              | 1.2              | 24.1%              | 5.1%           | 7.9%             | 6.6%             | 6.0%              |
| RivaGAN      | Trustmark Q (0.95) | -              | series   | -    | 132                | 67.2%    | 38.0              | 1.2              | 65.0%              | 16.3%          | 22.4%            | 20.9%            | 19.8%             |
| RoSteALS     | DwtDet             | -              | series   | 0.5  | 132                | 13.4%    | 34.8              | 3.3              | 3.7%               | 1.1%           | 0.0%             | 0.0%             | 0.0%              |
| RoSteALS     | DwtDet             | -              | series   | -    | 132                | 36.8%    | 30.4              | 3.4              | 9.7%               | 4.6%           | 0.0%             | 0.0%             | 0.0%              |
| RoSteALS     | DwtDetSvd          | -              | series   | 0.5  | 132                | 16.0%    | 34.8              | 3.4              | 4.2%               | 2.7%           | 0.0%             | 0.0%             | 0.0%              |
| RoSteALS     | DwtDetSvd          | -              | series   | -    | 132                | 65.1%    | 30.4              | 3.4              | 16.1%              | 11.3%          | 0.0%             | 0.1%             | 0.0%              |
| RoSteALS     | HiDDeN             | LC[148,102,14] | series   | 1    | 102                | 21.5%    | 33.3              | 4.0              | 8.2%               | 3.2%           | 0.0%             | 0.0%             | 0.0%              |
| RoSteALS     | HiDDeN             | LC[148,49,34]  | parallel | -0.2 | 49                 | 60.0%    | 34.5              | 3.7              | 28.2%              | 10.5%          | 0.1%             | 0.0%             | 0.0%              |
| RoSteALS     | HiDDeN             | LC[148,49,34]  | parallel | -0.1 | 49                 | 60.0%    | 34.5              | 3.7              | 28.1%              | 10.9%          | 0.1%             | 0.0%             | 0.0%              |
| RoSteALS     | HiDDeN             | LC[148,49,34]  | parallel | 0    | 49                 | 60.0%    | 34.5              | 3.7              | 26.4%              | 10.2%          | 0.0%             | 0.0%             | 0.0%              |
| RoSteALS     | HiDDeN             | LC[148,49,34]  | parallel | 0.1  | 49                 | 60.0%    | 34.5              | 3.7              | 26.2%              | 10.6%          | 0.1%             | 0.0%             | 0.0%              |
| RoSteALS     | HiDDeN             | LC[148,49,34]  | parallel | 0.2  | 49                 | 60.0%    | 34.5              | 3.7              | 25.4%              | 10.6%          | 0.0%             | 0.0%             | 0.0%              |
| RoSteALS     | HiDDeN             | LC[148,49,34]  | parallel | 0.3  | 49                 | 60.0%    | 34.5              | 3.7              | 27.1%              | 9.6%           | 0.0%             | 0.1%             | 0.0%              |
| RoSteALS     | HiDDeN             | LC[148,49,34]  | parallel | 0.4  | 49                 | 60.0%    | 34.5              | 3.7              | 27.0%              | 11.7%          | 0.0%             | 0.0%             | 0.1%              |
| RoSteALS     | HiDDeN             | LC[148,49,34]  | parallel | 0.5  | 49                 | 60.0%    | 34.5              | 3.7              | 25.6%              | 10.1%          | 0.1%             | 0.0%             | 0.1%              |
| RoSteALS     | HiDDeN             | LC[148,49,34]  | parallel | 0.6  | 49                 | 60.0%    | 34.5              | 3.7              | 26.4%              | 11.7%          | 0.0%             | 0.0%             | 0.0%              |
| RoSteALS     | HiDDeN             | LC[148,49,34]  | parallel | 0.7  | 49                 | 59.9%    | 34.5              | 3.7              | 25.4%              | 10.4%          | 0.0%             | 0.1%             | 0.0%              |
| RoSteALS     | HiDDeN             | LC[148,49,34]  | parallel | 0.8  | 49                 | 59.9%    | 34.5              | 3.7              | 25.6%              | 10.0%          | 0.2%             | 0.1%             | 0.0%              |
| RoSteALS     | HiDDeN             | LC[148,49,34]  | parallel | 0.9  | 49                 | 59.4%    | 34.6              | 3.7              | 27.2%              | 10.8%          | 0.0%             | 0.0%             | 0.0%              |
| RoSteALS     | HiDDeN             | LC[148,49,34]  | parallel | 1    | 49                 | 58.6%    | 34.7              | 3.7              | 25.3%              | 10.1%          | 0.0%             | 0.1%             | 0.0%              |
| RoSteALS     | HiDDeN             | LC[148,49,34]  | parallel | 1.1  | 49                 | 58.0%    | 34.8              | 3.8              | 25.0%              | 10.4%          | 0.0%             | 0.0%             | 0.1%              |
| RoSteALS     | HiDDeN             | LC[148,49,34]  | parallel | 1.2  | 49                 | 57.3%    | 34.9              | 3.8              | 25.3%              | 9.0%           | 0.0%             | 0.0%             | 0.1%              |
| RoSteALS     | HiDDeN             | LC[148,49,34]  | parallel | -    | 49                 | 60.0%    | 34.5              | 3.7              | 25.7%              | 11.6%          | 0.0%             | 0.0%             | 0.0%              |
| RoSteALS     | HiDDeN             | LC[148,49,34]  | series   | -0.2 | 49                 | 91.9%    | 30.2              | 3.8              | 45.6%              | 20.2%          | 0.2%             | 0.2%             | 0.0%              |
| RoSteALS     | HiDDeN             | LC[148,49,34]  | series   | -0.1 | 49                 | 91.0%    | 30.4              | 3.8              | 44.2%              | 19.1%          | 0.1%             | 0.2%             | 0.0%              |
| RoSteALS     | HiDDeN             | LC[148,49,34]  | series   | 0    | 49                 | 89.9%    | 30.7              | 3.8              | 43.2%              | 19.2%          | 0.3%             | 0.2%             | 0.1%              |
| RoSteALS     | HiDDeN             | LC[148,49,34]  | series   | 0.1  | 49                 | 89.4%    | 31.0              | 3.8              | 41.0%              | 21.6%          | 0.1%             | 0.1%             | 0.1%              |
| RoSteALS     | HiDDeN             | LC[148,49,34]  | series   | 0.2  | 49                 | 88.3%    | 31.2              | 3.7              | 44.1%              | 19.5%          | 0.2%             | 0.1%             | 0.3%              |
| RoSteALS     | HiDDeN             | LC[148,49,34]  | series   | 0.3  | 49                 | 87.0%    | 31.5              | 3.8              | 41.2%              | 19.4%          | 0.1%             | 0.1%             | 0.0%              |
| RoSteALS     | HiDDeN             | LC[148,49,34]  | series   | 0.4  | 49                 | 85.1%    | 31.7              | 3.8              | 42.4%              | 17.7%          | 0.1%             | 0.0%             | 0.2%              |
| RoSteALS     | HiDDeN             | LC[148,49,34]  | series   | 0.5  | 49                 | 81.6%    | 32.0              | 3.8              | 38.9%              | 17.6%          | 0.1%             | 0.2%             | 0.1%              |
| RoSteALS     | HiDDeN             | LC[148,49,34]  | series   | 0.6  | 49                 | 79.7%    | 32.3              | 3.8              | 37.8%              | 16.1%          | 0.1%             | 0.1%             | 0.0%              |
| RoSteALS     | HiDDeN             | LC[148,49,34]  | series   | 0.7  | 49                 | 78.4%    | 32.5              | 3.8              | 37.0%              | 15.5%          | 0.2%             | 0.1%             | 0.0%              |
| RoSteALS     | HiDDeN             | LC[148,49,34]  | series   | 0.8  | 49                 | 75.6%    | 32.8              | 3.9              | 36.8%              | 15.4%          | 0.0%             | 0.1%             | 0.2%              |
| RoSteALS     | HiDDeN             | LC[148,49,34]  | series   | 0.9  | 49                 | 73.3%    | 33.0              | 4.0              | 34.7%              | 14.6%          | 0.0%             | 0.0%             | 0.2%              |
| RoSteALS     | HiDDeN             | LC[148,49,34]  | series   | 1    | 49                 | 72.2%    | 33.3              | 4.0              | 34.5%              | 14.4%          | 0.2%             | 0.0%             | 0.0%              |
| RoSteALS     | HiDDeN             | LC[148,49,34]  | series   | 1.1  | 49                 | 69.4%    | 33.5              | 4.1              | 35.1%              | 13.1%          | 0.1%             | 0.2%             | 0.0%              |
| RoSteALS     | HiDDeN             | LC[148,49,34]  | series   | 1.2  | 49                 | 66.8%    | 33.8              | 4.2              | 30.1%              | 12.7%          | 0.1%             | 0.0%             | 0.0%              |
| RoSteALS     | HiDDeN             | LC[148,49,34]  | series   | -    | 49                 | 94.9%    | 28.7              | 3.8              | 47.1%              | 24.5%          | 0.2%             | 0.3%             | 0.2%              |
| RoSteALS     | HiDDeN             | -              | parallel | 0.5  | 148                | 0.0%     | 34.5              | 3.7              | 0.0%               | 0.0%           | 0.0%             | 0.0%             | 0.0%              |
| RoSteALS     | HiDDeN             | -              | parallel | -    | 148                | 0.0%     | 34.5              | 3.7              | 0.0%               | 0.0%           | 0.0%             | 0.0%             | 0.0%              |
| RoSteALS     | HiDDeN             | -              | series   | 0.5  | 148                | 0.2%     | 32.0              | 3.8              | 0.0%               | 0.0%           | 0.0%             | 0.0%             | 0.0%              |
| RoSteALS     | HiDDeN             | -              | series   | -    | 148                | 7.0%     | 28.7              | 3.8              | 1.9%               | 1.1%           | 0.0%             | 0.0%             | 0.0%              |
| RoSteALS     | -                  | LC[100,32,25]  | -        | -    | 32                 | 99.9%    | 31.4              | 3.6              | 50.4%              | 31.7%          | 0.4%             | 0.5%             | 0.5%              |
| RoSteALS     | -                  | LC[100,48,20]  | -        | -    | 48                 | 99.9%    | 31.4              | 3.6              | 50.0%              | 31.6%          | 0.3%             | 0.4%             | 0.4%              |
| RoSteALS     | -                  | -              | -        | -    | 100                | 72.1%    | 31.4              | 3.6              | 35.4%              | 22.1%          | 0.1%             | 0.1%             | 0.1%              |
| RoSteALS     | RivaGAN            | LC[131,32,37]  | series   | -0.2 | 32                 | 99.9%    | 30.8              | 3.4              | 50.0%              | 30.6%          | 0.5%             | 0.8%             | 0.5%              |
| RoSteALS     | RivaGAN            | LC[131,32,37]  | series   | -0.1 | 32                 | 99.8%    | 30.9              | 3.5              | 52.2%              | 30.5%          | 0.4%             | 0.7%             | 0.5%              |
| RoSteALS     | RivaGAN            | LC[131,32,37]  | series   | 0    | 32                 | 99.9%    | 31.3              | 3.6              | 51.7%              | 31.2%          | 0.5%             | 0.4%             | 0.3%              |
| RoSteALS     | RivaGAN            | LC[131,32,37]  | series   | 0.1  | 32                 | 99.8%    | 32.3              | 3.3              | 51.8%              | 32.0%          | 0.4%             | 0.4%             | 0.6%              |
| RoSteALS     | RivaGAN            | LC[131,32,37]  | series   | 0.2  | 32                 | 99.5%    | 33.2              | 2.9              | 51.9%              | 31.2%          | 0.6%             | 0.3%             | 0.3%              |
| RoSteALS     | RivaGAN            | LC[131,32,37]  | series   | 0.3  | 32                 | 98.8%    | 34.2              | 2.6              | 50.0%              | 30.8%          | 0.5%             | 0.4%             | 0.2%              |
| RoSteALS     | RivaGAN            | LC[131,32,37]  | series   | 0.4  | 32                 | 97.1%    | 35.1              | 2.2              | 49.2%              | 29.6%          | 0.3%             | 0.3%             | 0.4%              |
| RoSteALS     | RivaGAN            | LC[131,32,37]  | series   | 0.5  | 32                 | 94.4%    | 36.1              | 1.9              | 48.9%              | 27.5%          | 0.3%             | 0.3%             | 0.1%              |

| First method       | Second method      | ECC            | Ensemble | Clip | Capacity (bits) | Accuracy | Mean PSNR [dB] | Std PSNR [dB] | Robust. RivaGAN | Robust. SSL | Robust. TmLow | Robust. TmMed | Robust. TmHigh |
|--------------------|--------------------|----------------|----------|------|-----------------|----------|----------------|---------------|-----------------|-------------|---------------|---------------|----------------|
| RoSteALS           | RivaGAN            | LC[131,32,37]  | series   | 0.6  | 32              | 88.7%    | 37.0           | 1.6           | 43.0%           | 24.3%       | 0.0%          | 0.2%          | 0.1%           |
| RoSteALS           | RivaGAN            | LC[131,32,37]  | series   | 0.7  | 32              | 83.2%    | 38.0           | 1.2           | 43.3%           | 22.1%       | 0.1%          | 0.1%          | 0.1%           |
| RoSteALS           | RivaGAN            | LC[131,32,37]  | series   | 0.8  | 32              | 77.9%    | 38.9           | 1.0           | 40.1%           | 22.3%       | 0.1%          | 0.2%          | 0.1%           |
| RoSteALS           | RivaGAN            | LC[131,32,37]  | series   | 0.9  | 32              | 71.4%    | 39.9           | 0.8           | 37.4%           | 19.4%       | 0.0%          | 0.1%          | 0.2%           |
| RoSteALS           | RivaGAN            | LC[131,32,37]  | series   | 1    | 32              | 64.7%    | 40.8           | 0.7           | 33.7%           | 16.8%       | 0.1%          | 0.1%          | 0.1%           |
| RoSteALS           | RivaGAN            | LC[131,32,37]  | series   | 1.1  | 32              | 55.3%    | 41.8           | 0.7           | 27.0%           | 15.8%       | 0.2%          | 0.0%          | 0.1%           |
| RoSteALS           | RivaGAN            | LC[131,32,37]  | series   | 1.2  | 32              | 49.2%    | 42.7           | 0.9           | 23.9%           | 14.8%       | 0.1%          | 0.2%          | 0.1%           |
| RoSteALS           | RivaGAN            | LC[131,32,37]  | series   | -    | 32              | 99.9%    | 30.7           | 3.1           | 54.6%           | 28.3%       | 0.5%          | 0.4%          | 0.5%           |
| RoSteALS           | RivaGAN            | -              | series   | 0.5  | 132             | 8.0%     | 36.1           | 1.9           | 4.0%            | 1.8%        | 0.0%          | 0.0%          | 0.0%           |
| RoSteALS           | RivaGAN            | -              | series   | -    | 132             | 42.9%    | 30.7           | 3.1           | 22.5%           | 9.3%        | 0.0%          | 0.0%          | 0.0%           |
| RoSteALS           | RoSteALS           | -              | parallel | 0.5  | 200             | 0.0%     | 32.2           | 3.6           | 0.0%            | 0.0%        | 0.0%          | 0.0%          | 0.0%           |
| RoSteALS           | RoSteALS           | -              | parallel | -    | 200             | 0.0%     | 32.2           | 3.6           | 0.0%            | 0.0%        | 0.0%          | 0.0%          | 0.0%           |
| RoSteALS           | RoSteALS           | -              | series   | 0.5  | 200             | 0.0%     | 31.3           | 3.6           | 0.0%            | 0.0%        | 0.0%          | 0.0%          | 0.0%           |
| RoSteALS           | RoSteALS           | -              | series   | -    | 200             | 0.0%     | 27.8           | 3.2           | 0.0%            | 0.0%        | 0.0%          | 0.0%          | 0.0%           |
| RoSteALS           | SSL (42dB,30bits)  | LC[130,100,10] | series   | 0.2  | 100             | 86.8%    | 33.5           | 2.9           | 43.8%           | 21.6%       | 0.4%          | 0.1%          | 0.0%           |
| RoSteALS           | SSL (42dB,30bits)  | -              | series   | 0.5  | 130             | 20.0%    | 36.7           | 1.9           | 8.3%            | 4.0%        | 0.0%          | 0.1%          | 0.0%           |
| RoSteALS           | SSL (42dB,30bits)  | -              | series   | -    | 130             | 66.8%    | 30.9           | 3.3           | 32.5%           | 16.6%       | 0.0%          | 0.1%          | 0.1%           |
| RoSteALS           | Trustmark B (0.95) | -              | parallel | 0.5  | 200             | 4.6%     | 36.6           | 3.0           | 1.8%            | 1.0%        | 0.0%          | 0.0%          | 0.0%           |
| RoSteALS           | Trustmark B (0.95) | -              | parallel | -    | 200             | 4.7%     | 36.4           | 3.2           | 2.7%            | 1.6%        | 0.0%          | 0.0%          | 0.0%           |
| RoSteALS           | Trustmark B (0.95) | -              | series   | 0.5  | 200             | 5.8%     | 36.3           | 2.7           | 2.6%            | 1.9%        | 0.0%          | 0.0%          | 0.0%           |
| RoSteALS           | Trustmark B (0.95) | -              | series   | -    | 200             | 48.5%    | 30.8           | 3.3           | 25.7%           | 14.7%       | 0.0%          | 0.1%          | 0.0%           |
| RoSteALS           | Trustmark Q (0.95) | -              | parallel | 0.5  | 200             | 2.5%     | 36.9           | 2.9           | 1.2%            | 0.6%        | 0.0%          | 0.0%          | 0.0%           |
| RoSteALS           | Trustmark Q (0.95) | -              | parallel | -    | 200             | 3.0%     | 36.5           | 3.2           | 1.6%            | 0.8%        | 0.0%          | 0.0%          | 0.0%           |
| RoSteALS           | Trustmark Q (0.95) | -              | series   | 0.5  | 200             | 5.3%     | 36.8           | 2.8           | 3.1%            | 1.2%        | 0.0%          | 0.0%          | 0.0%           |
| RoSteALS           | Trustmark Q (0.95) | -              | series   | -    | 200             | 50.2%    | 30.8           | 3.4           | 24.9%           | 16.5%       | 0.0%          | 0.2%          | 0.0%           |
| SSL (42dB,30bits)  | DwtDct             | -              | parallel | 0.5  | 62              | 9.4%     | 42.3           | 2.6           | 2.7%            | 0.9%        | 0.0%          | 0.0%          | 0.0%           |
| SSL (42dB,30bits)  | DwtDct             | -              | parallel | -    | 62              | 9.4%     | 42.3           | 2.7           | 2.3%            | 0.9%        | 0.0%          | 0.0%          | 0.0%           |
| SSL (42dB,30bits)  | DwtDct             | -              | series   | 0.5  | 62              | 25.6%    | 40.2           | 2.1           | 7.1%            | 3.3%        | 0.0%          | 0.0%          | 0.0%           |
| SSL (42dB,30bits)  | DwtDct             | -              | series   | -    | 62              | 32.0%    | 36.5           | 2.8           | 7.8%            | 2.8%        | 0.0%          | 0.0%          | 0.0%           |
| SSL (42dB,30bits)  | DwtDctSvd          | -              | parallel | 0.5  | 62              | 21.5%    | 42.2           | 2.5           | 6.1%            | 2.2%        | 0.0%          | 0.0%          | 0.0%           |
| SSL (42dB,30bits)  | DwtDctSvd          | -              | parallel | -    | 62              | 21.5%    | 42.1           | 2.7           | 5.1%            | 1.9%        | 0.0%          | 0.0%          | 0.0%           |
| SSL (42dB,30bits)  | DwtDctSvd          | -              | series   | 0.5  | 62              | 46.8%    | 40.2           | 2.1           | 12.3%           | 6.9%        | 0.0%          | 0.0%          | 0.1%           |
| SSL (42dB,30bits)  | DwtDctSvd          | -              | series   | -    | 62              | 64.0%    | 36.4           | 2.8           | 15.4%           | 9.2%        | 0.0%          | 0.1%          | 0.0%           |
| SSL (42dB,30bits)  | HiDDeN             | -              | parallel | 0.5  | 78              | 0.1%     | 38.3           | 3.1           | 0.0%            | 0.0%        | 0.0%          | 0.0%          | 0.0%           |
| SSL (42dB,30bits)  | HiDDeN             | -              | parallel | -    | 78              | 0.3%     | 37.9           | 3.8           | 0.0%            | 0.0%        | 0.0%          | 0.0%          | 0.0%           |
| SSL (42dB,30bits)  | HiDDeN             | -              | series   | 0.5  | 78              | 0.1%     | 37.4           | 2.3           | 0.0%            | 0.0%        | 0.0%          | 0.0%          | 0.0%           |
| SSL (42dB,30bits)  | HiDDeN             | -              | series   | -    | 78              | 5.1%     | 32.0           | 3.9           | 1.4%            | 0.6%        | 0.0%          | 0.0%          | 0.0%           |
| SSL (42dB,30bits)  | -                  | -              | -        | -    | 30              | 93.8%    | 42.1           | 0.6           | 86.1%           | 75.8%       | 58.0%         | 52.2%         | 47.9%          |
| SSL (42dB,30bits)  | RivaGAN            | -              | parallel | 0.5  | 62              | 27.8%    | 43.7           | 0.5           | 11.6%           | 4.3%        | 1.5%          | 1.0%          | 1.1%           |
| SSL (42dB,30bits)  | RivaGAN            | -              | parallel | -    | 62              | 27.8%    | 43.7           | 0.5           | 10.7%           | 4.3%        | 0.9%          | 1.0%          | 0.4%           |
| SSL (42dB,30bits)  | RivaGAN            | -              | series   | 0.5  | 62              | 53.4%    | 41.5           | 0.6           | 32.8%           | 12.8%       | 6.1%          | 4.2%          | 3.7%           |
| SSL (42dB,30bits)  | RivaGAN            | -              | series   | -    | 62              | 64.5%    | 38.4           | 0.5           | 51.4%           | 17.5%       | 11.7%         | 10.8%         | 8.2%           |
| SSL (42dB,30bits)  | RoSteALS           | -              | parallel | 0.5  | 130             | 8.0%     | 37.3           | 2.5           | 2.7%            | 1.4%        | 0.0%          | 0.0%          | 0.0%           |
| SSL (42dB,30bits)  | RoSteALS           | -              | parallel | -    | 130             | 8.2%     | 36.8           | 3.2           | 3.1%            | 1.2%        | 0.0%          | 0.0%          | 0.0%           |
| SSL (42dB,30bits)  | RoSteALS           | -              | series   | 0.5  | 130             | 2.3%     | 36.7           | 1.9           | 0.7%            | 0.4%        | 0.0%          | 0.0%          | 0.0%           |
| SSL (42dB,30bits)  | RoSteALS           | -              | series   | -    | 130             | 15.6%    | 30.9           | 3.3           | 5.7%            | 2.2%        | 0.0%          | 0.0%          | 0.0%           |
| SSL (42dB,30bits)  | SSL (42dB,30bits)  | -              | parallel | 0.5  | 60              | 0.0%     | 44.2           | 0.6           | 0.0%            | 0.0%        | 0.0%          | 0.0%          | 0.0%           |
| SSL (42dB,30bits)  | SSL (42dB,30bits)  | -              | parallel | -    | 60              | 0.0%     | 44.2           | 0.6           | 0.0%            | 0.0%        | 0.0%          | 0.0%          | 0.0%           |
| SSL (42dB,30bits)  | SSL (42dB,30bits)  | -              | series   | 0.5  | 60              | 0.0%     | 42.1           | 0.6           | 0.0%            | 0.0%        | 0.0%          | 0.0%          | 0.0%           |
| SSL (42dB,30bits)  | SSL (42dB,30bits)  | -              | series   | 0.5  | 60              | 0.0%     | 42.1           | 0.6           | 0.0%            | 0.0%        | 0.0%          | 0.0%          | 0.0%           |
| SSL (42dB,30bits)  | SSL (42dB,30bits)  | -              | series   | -    | 60              | 0.0%     | 39.1           | 0.6           | 0.0%            | 0.0%        | 0.0%          | 0.0%          | 0.0%           |
| SSL (42dB,30bits)  | SSL (42dB,30bits)  | -              | series   | -    | 60              | 0.0%     | 39.1           | 0.6           | 0.0%            | 0.0%        | 0.0%          | 0.0%          | 0.0%           |
| SSL (42dB,30bits)  | Trustmark B (0.95) | -              | parallel | 0.5  | 130             | 5.3%     | 43.8           | 1.1           | 2.8%            | 1.6%        | 1.2%          | 0.8%          | 0.5%           |
| SSL (42dB,30bits)  | Trustmark B (0.95) | -              | parallel | -    | 130             | 5.3%     | 43.8           | 1.1           | 3.1%            | 1.6%        | 1.4%          | 0.8%          | 0.7%           |
| SSL (42dB,30bits)  | Trustmark B (0.95) | -              | series   | 0.5  | 130             | 35.4%    | 41.7           | 1.0           | 28.2%           | 16.3%       | 13.8%         | 12.3%         | 9.5%           |
| SSL (42dB,30bits)  | Trustmark B (0.95) | -              | series   | -    | 130             | 77.7%    | 38.4           | 1.2           | 68.8%           | 41.5%       | 43.0%         | 36.7%         | 32.7%          |
| SSL (42dB,30bits)  | Trustmark Q (0.95) | -              | parallel | 0.5  | 130             | 2.5%     | 44.3           | 1.1           | 2.0%            | 1.2%        | 0.5%          | 0.5%          | 0.4%           |
| SSL (42dB,30bits)  | Trustmark Q (0.95) | -              | parallel | -    | 130             | 2.5%     | 44.3           | 1.1           | 2.1%            | 1.0%        | 0.4%          | 0.5%          | 0.5%           |
| SSL (42dB,30bits)  | Trustmark Q (0.95) | -              | series   | 0.5  | 130             | 35.2%    | 42.3           | 1.2           | 28.3%           | 14.2%       | 13.4%         | 11.1%         | 9.0%           |
| SSL (42dB,30bits)  | Trustmark Q (0.95) | -              | series   | -    | 130             | 77.3%    | 39.0           | 1.2           | 66.8%           | 37.6%       | 40.5%         | 34.9%         | 31.8%          |
| Trustmark B (0.95) | DwtDct             | -              | series   | 0.5  | 132             | 20.5%    | 39.7           | 2.4           | 4.7%            | 2.5%        | 0.0%          | 0.0%          | 0.0%           |
| Trustmark B (0.95) | DwtDct             | -              | series   | -    | 132             | 49.3%    | 36.2           | 2.8           | 11.3%           | 5.4%        | 0.1%          | 0.0%          | 0.0%           |
| Trustmark B (0.95) | DwtDctSvd          | -              | series   | 0.5  | 132             | 26.7%    | 39.7           | 2.5           | 6.4%            | 4.2%        | 0.1%          | 0.0%          | 0.0%           |
| Trustmark B (0.95) | DwtDctSvd          | -              | series   | -    | 132             | 88.5%    | 36.0           | 2.8           | 23.3%           | 16.4%       | 0.3%          | 0.1%          | 0.4%           |
| Trustmark B (0.95) | HiDDeN             | -              | series   | 0.5  | 148             | 0.0%     | 36.9           | 3.0           | 0.0%            | 0.0%        | 0.0%          | 0.0%          | 0.0%           |
| Trustmark B (0.95) | HiDDeN             | -              | series   | -    | 148             | 13.2%    | 31.9           | 4.0           | 4.8%            | 1.4%        | 0.0%          | 0.0%          | 0.1%           |
| Trustmark B (0.95) | -                  | -              | -        | -    | 100             | 96.5%    | 41.3           | 2.1           | 96.9%           | 67.9%       | 85.2%         | 83.1%         | 79.4%          |
| Trustmark B (0.95) | RivaGAN            | -              | series   | 0.5  | 132             | 24.3%    | 40.9           | 1.1           | 27.2%           | 6.2%        | 9.4%          | 8.5%          | 6.6%           |
| Trustmark B (0.95) | RivaGAN            | -              | series   | -    | 132             | 73.9%    | 37.5           | 1.1           | 72.6%           | 20.1%       | 26.7%         | 26.7%         | 21.4%          |
| Trustmark B (0.95) | RoSteALS           | -              | series   | 0.5  | 200             | 4.2%     | 36.2           | 2.7           | 1.9%            | 1.1%        | 0.0%          | 0.0%          | 0.0%           |
| Trustmark B (0.95) | RoSteALS           | -              | series   | -    | 200             | 31.1%    | 30.7           | 3.3           | 15.6%           | 9.1%        | 0.0%          | 0.0%          | 0.0%           |
| Trustmark B (0.95) | SSL (42dB,100bits) | LC[200,100,32] | series   | 1    | 100             | 80.6%    | 42.5           | 1.1           | 67.4%           | 39.3%       | 40.8%         | 37.9%         | 32.9%          |
| Trustmark B (0.95) | SSL (42dB,100bits) | -              | series   | 1    | 200             | 22.9%    | 42.5           | 1.1           | 11.4%           | 6.2%        | 2.1%          | 2.6%          | 2.4%           |
| Trustmark B (0.95) | SSL (42dB,30bits)  | -              | series   | 0.5  | 130             | 45.7%    | 41.7           | 1.0           | 42.8%           | 22.4%       | 21.9%         | 20.2%         | 18.1%          |
| Trustmark B (0.95) | SSL (42dB,30bits)  | -              | series   | -    | 130             | 92.9%    | 38.4           | 1.1           | 88.7%           | 54.1%       | 61.1%         | 53.8%         | 48.6%          |
| Trustmark B (0.95) | Trustmark B (0.95) | -              | parallel | 0.5  | 200             | 0.0%     | 42.0           | 2.1           | 0.0%            | 0.0%        | 0.0%          | 0.0%          | 0.0%           |
| Trustmark B (0.95) | Trustmark B (0.95) | -              | parallel | -    | 200             | 0.0%     | 42.0           | 2.1           | 0.0%            | 0.0%        | 0.0%          | 0.0%          | 0.0%           |
| Trustmark B (0.95) | Trustmark B (0.95) | -              | series   | 0.5  | 200             | 0.0%     | 41.4           | 2.2           | 0.0%            | 0.0%        | 0.0%          | 0.0%          | 0.0%           |
| Trustmark B (0.95) | Trustmark B (0.95) | -              | series   | -    | 200             | 0.0%     | 38.0           | 2.1           | 0.0%            | 0.0%        | 0.0%          | 0.0%          | 0.0%           |
| Trustmark B (0.95) | Trustmark Q (0.95) | -              | series   | 0.5  | 200             | 0.1%     | 41.9           | 2.2           | 0.1%            | 0.0%        | 0.0%          | 0.0%          | 0.0%           |
| Trustmark B (0.95) | Trustmark Q (0.95) | -              | series   | -    | 200             | 0.1%     | 38.6           | 2.3           | 0.2%            | 0.0%        | 0.0%          | 0.0%          | 0.0%           |
| Trustmark Q (0.40) | -                  | LC[100,32,25]  | -        | -    | 32              | 49.6%    | 47.9           | 1.8           | 54.0%           | 30.7%       | 40.5%         | 38.3%         | 36.0%          |
| Trustmark Q (0.45) | -                  | LC[100,32,25]  | -        | -    | 32              | 65.5%    | 47.3           | 1.9           | 70.5%           | 41.3%       | 54.9%         | 51.7%         | 48.5%          |
| Trustmark Q (0.50) | -                  | LC[100,32,25]  | -        | -    | 32              | 80.2%    | 46.8           | 2.0           | 83.5%           | 51.8%       | 68.4%         | 64.3%         | 60.9%          |
| Trustmark Q (0.55) | -                  | LC[100,32,25]  | -        | -    | 32              | 88.9%    | 46.2           | 2.0           | 91.0%           | 58.7%       | 77.1%         | 73.8%         | 70.5%          |
| Trustmark Q (0.60) | -                  | LC[100,32,25]  | -        | -    | 32              | 95.1%    | 45.7           | 2.1           | 95.9%           | 64.0%       | 83.2%         | 81.3%         | 76.7%          |

| First method       | Second method      | ECC           | Ensemble | Clip | Capacity<br>(bits) | Accuracy | Mean<br>PSNR [dB] | Std<br>PSNR [dB] | Robust.<br>RivaGAN | Robust.<br>SSL | Robust.<br>TmLow | Robust.<br>TmMed | Robust.<br>TmHigh |
|--------------------|--------------------|---------------|----------|------|--------------------|----------|-------------------|------------------|--------------------|----------------|------------------|------------------|-------------------|
| Trustmark Q (0.60) | RivaGAN            | LC[131,32,37] | series   | -0.2 | 32                 | 85.3%    | 39.8              | 0.9              | 86.5%              | 38.7%          | 52.4%            | 49.2%            | 46.9%             |
| Trustmark Q (0.60) | RivaGAN            | LC[131,32,37] | series   | -0.1 | 32                 | 81.7%    | 40.1              | 0.8              | 83.5%              | 36.3%          | 48.6%            | 45.7%            | 41.8%             |
| Trustmark Q (0.60) | RivaGAN            | LC[131,32,37] | series   | 0    | 32                 | 75.3%    | 40.7              | 0.7              | 78.5%              | 33.0%          | 42.1%            | 39.8%            | 36.5%             |
| Trustmark Q (0.60) | RivaGAN            | LC[131,32,37] | series   | 0.1  | 32                 | 69.9%    | 41.3              | 0.6              | 72.7%              | 28.0%          | 36.0%            | 34.1%            | 31.3%             |
| Trustmark Q (0.60) | RivaGAN            | LC[131,32,37] | series   | 0.2  | 32                 | 63.6%    | 41.7              | 0.8              | 67.4%              | 22.6%          | 32.1%            | 30.6%            | 25.4%             |
| Trustmark Q (0.60) | RivaGAN            | LC[131,32,37] | series   | 0.3  | 32                 | 58.3%    | 42.2              | 0.9              | 62.8%              | 22.3%          | 26.8%            | 26.0%            | 23.7%             |
| Trustmark Q (0.60) | RivaGAN            | LC[131,32,37] | series   | 0.4  | 32                 | 51.0%    | 42.6              | 1.0              | 55.0%              | 17.0%          | 23.5%            | 21.4%            | 18.5%             |
| Trustmark Q (0.60) | RivaGAN            | LC[131,32,37] | series   | 0.5  | 32                 | 41.3%    | 43.2              | 1.2              | 44.0%              | 13.1%          | 17.1%            | 15.7%            | 15.9%             |
| Trustmark Q (0.60) | RivaGAN            | LC[131,32,37] | series   | 0.6  | 32                 | 35.1%    | 43.6              | 1.3              | 39.6%              | 12.4%          | 15.5%            | 14.2%            | 12.4%             |
| Trustmark Q (0.60) | RivaGAN            | LC[131,32,37] | series   | 0.7  | 32                 | 33.0%    | 44.0              | 1.5              | 37.6%              | 11.0%          | 14.2%            | 13.1%            | 12.8%             |
| Trustmark Q (0.60) | RivaGAN            | LC[131,32,37] | series   | 0.8  | 32                 | 29.5%    | 44.6              | 1.8              | 33.6%              | 9.7%           | 11.8%            | 11.3%            | 10.6%             |
| Trustmark Q (0.60) | RivaGAN            | LC[131,32,37] | series   | 0.9  | 32                 | 26.5%    | 45.1              | 2.0              | 27.9%              | 8.3%           | 9.9%             | 9.1%             | 7.9%              |
| Trustmark Q (0.60) | RivaGAN            | LC[131,32,37] | series   | 1    | 32                 | 22.5%    | 45.6              | 2.1              | 23.5%              | 6.7%           | 8.5%             | 7.7%             | 6.2%              |
| Trustmark Q (0.60) | RivaGAN            | LC[131,32,37] | series   | 1.1  | 32                 | 17.7%    | 46.0              | 2.3              | 17.8%              | 5.0%           | 6.9%             | 5.5%             | 5.0%              |
| Trustmark Q (0.60) | RivaGAN            | LC[131,32,37] | series   | 1.2  | 32                 | 14.3%    | 46.5              | 2.4              | 14.8%              | 4.7%           | 5.0%             | 5.3%             | 4.7%              |
| Trustmark Q (0.60) | RivaGAN            | LC[131,32,37] | series   | -    | 32                 | 94.2%    | 39.0              | 0.8              | 95.0%              | 46.1%          | 59.8%            | 57.7%            | 53.2%             |
| Trustmark Q (0.65) | -                  | LC[100,32,25] | -        | -    | 32                 | 97.8%    | 45.2              | 2.1              | 98.0%              | 65.1%          | 87.1%            | 85.0%            | 82.8%             |
| Trustmark Q (0.70) | -                  | LC[100,32,25] | -        | -    | 32                 | 98.7%    | 44.7              | 2.2              | 98.8%              | 66.8%          | 89.2%            | 87.6%            | 85.6%             |
| Trustmark Q (0.75) | -                  | LC[100,32,25] | -        | -    | 32                 | 99.6%    | 44.2              | 2.2              | 99.5%              | 68.9%          | 89.8%            | 88.8%            | 86.7%             |
| Trustmark Q (0.80) | -                  | LC[100,32,25] | -        | -    | 32                 | 99.6%    | 43.7              | 2.3              | 99.5%              | 69.7%          | 90.9%            | 89.1%            | 87.6%             |
| Trustmark Q (0.80) | RivaGAN            | LC[131,32,37] | series   | -0.2 | 32                 | 95.9%    | 39.9              | 0.9              | 96.5%              | 50.5%          | 66.5%            | 63.8%            | 61.6%             |
| Trustmark Q (0.80) | RivaGAN            | LC[131,32,37] | series   | -0.1 | 32                 | 95.6%    | 40.3              | 0.9              | 96.1%              | 47.3%          | 63.5%            | 61.1%            | 59.0%             |
| Trustmark Q (0.80) | RivaGAN            | LC[131,32,37] | series   | 0    | 32                 | 95.4%    | 40.6              | 0.8              | 96.1%              | 46.5%          | 62.1%            | 58.5%            | 55.4%             |
| Trustmark Q (0.80) | RivaGAN            | LC[131,32,37] | series   | 0.1  | 32                 | 93.7%    | 41.0              | 0.8              | 94.2%              | 47.1%          | 58.9%            | 56.6%            | 54.2%             |
| Trustmark Q (0.80) | RivaGAN            | LC[131,32,37] | series   | 0.2  | 32                 | 92.6%    | 41.3              | 0.8              | 94.1%              | 44.5%          | 57.3%            | 55.8%            | 52.3%             |
| Trustmark Q (0.80) | RivaGAN            | LC[131,32,37] | series   | 0.3  | 32                 | 92.2%    | 41.6              | 1.0              | 94.0%              | 42.8%          | 56.1%            | 53.3%            | 50.0%             |
| Trustmark Q (0.80) | RivaGAN            | LC[131,32,37] | series   | 0.4  | 32                 | 88.7%    | 41.9              | 1.1              | 90.6%              | 40.5%          | 52.1%            | 48.7%            | 45.3%             |
| Trustmark Q (0.80) | RivaGAN            | LC[131,32,37] | series   | 0.5  | 32                 | 86.0%    | 42.1              | 1.2              | 88.2%              | 37.3%          | 49.5%            | 44.5%            | 42.4%             |
| Trustmark Q (0.80) | RivaGAN            | LC[131,32,37] | series   | 0.6  | 32                 | 83.4%    | 42.5              | 1.4              | 86.6%              | 35.0%          | 46.1%            | 42.1%            | 39.3%             |
| Trustmark Q (0.80) | RivaGAN            | LC[131,32,37] | series   | 0.7  | 32                 | 81.3%    | 42.8              | 1.5              | 84.1%              | 32.1%          | 41.5%            | 39.4%            | 36.7%             |
| Trustmark Q (0.80) | RivaGAN            | LC[131,32,37] | series   | 0.8  | 32                 | 78.4%    | 43.1              | 1.7              | 80.9%              | 29.0%          | 40.7%            | 37.5%            | 34.4%             |
| Trustmark Q (0.80) | RivaGAN            | LC[131,32,37] | series   | 0.9  | 32                 | 74.3%    | 43.4              | 1.9              | 78.4%              | 28.0%          | 36.0%            | 33.5%            | 30.4%             |
| Trustmark Q (0.80) | RivaGAN            | LC[131,32,37] | series   | 1    | 32                 | 71.3%    | 43.7              | 2.1              | 74.2%              | 25.8%          | 34.0%            | 32.1%            | 28.8%             |
| Trustmark Q (0.80) | RivaGAN            | LC[131,32,37] | series   | 1.1  | 32                 | 66.6%    | 44.0              | 2.3              | 69.5%              | 24.5%          | 33.7%            | 28.3%            | 26.2%             |
| Trustmark Q (0.80) | RivaGAN            | LC[131,32,37] | series   | 1.2  | 32                 | 61.4%    | 44.4              | 2.5              | 65.1%              | 21.8%          | 27.6%            | 26.4%            | 22.8%             |
| Trustmark Q (0.80) | RivaGAN            | LC[131,32,37] | series   | -    | 32                 | 99.6%    | 38.4              | 1.0              | 99.7%              | 59.7%          | 75.2%            | 73.8%            | 71.6%             |
| Trustmark Q (0.85) | -                  | LC[100,32,25] | -        | -    | 32                 | 99.8%    | 43.3              | 2.3              | 99.6%              | 69.8%          | 91.3%            | 90.3%            | 89.0%             |
| Trustmark Q (0.90) | -                  | LC[100,32,25] | -        | -    | 32                 | 99.8%    | 42.9              | 2.3              | 99.6%              | 70.1%          | 91.4%            | 90.9%            | 89.0%             |
| Trustmark Q (0.95) | DwtDct             | -             | series   | 0.5  | 132                | 15.9%    | 40.3              | 2.5              | 3.9%               | 1.8%           | 0.0%             | 0.0%             | 0.0%              |
| Trustmark Q (0.95) | DwtDct             | -             | series   | -    | 132                | 48.4%    | 36.6              | 3.0              | 12.6%              | 6.1%           | 0.0%             | 0.0%             | 0.0%              |
| Trustmark Q (0.95) | DwtDctSvd          | -             | series   | 0.5  | 132                | 23.0%    | 40.3              | 2.6              | 6.5%               | 4.6%           | 0.0%             | 0.0%             | 0.0%              |
| Trustmark Q (0.95) | DwtDctSvd          | -             | series   | -    | 132                | 84.3%    | 36.4              | 3.0              | 19.5%              | 14.3%          | 0.2%             | 0.1%             | 0.2%              |
| Trustmark Q (0.95) | HiDDeN             | -             | series   | 0.5  | 148                | 0.0%     | 37.5              | 3.1              | 0.0%               | 0.0%           | 0.0%             | 0.0%             | 0.0%              |
| Trustmark Q (0.95) | HiDDeN             | -             | series   | -    | 148                | 11.4%    | 32.1              | 4.1              | 3.7%               | 1.5%           | 0.0%             | 0.0%             | 0.0%              |
| Trustmark Q (0.95) | -                  | LC[100,32,25] | -        | -    | 32                 | 99.9%    | 42.5              | 2.4              | 99.8%              | 70.3%          | 92.2%            | 90.9%            | 89.8%             |
| Trustmark Q (0.95) | -                  | -             | -        | -    | 100                | 93.7%    | 42.5              | 2.4              | 94.8%              | 62.6%          | 81.0%            | 77.8%            | 74.3%             |
| Trustmark Q (0.95) | RivaGAN            | LC[131,32,37] | series   | -0.2 | 32                 | 99.6%    | 39.9              | 1.1              | 99.5%              | 56.8%          | 73.8%            | 70.1%            | 68.2%             |
| Trustmark Q (0.95) | RivaGAN            | LC[131,32,37] | series   | -0.1 | 32                 | 99.4%    | 40.1              | 1.0              | 99.2%              | 53.9%          | 72.7%            | 69.7%            | 66.5%             |
| Trustmark Q (0.95) | RivaGAN            | LC[131,32,37] | series   | 0    | 32                 | 99.1%    | 40.4              | 1.0              | 99.2%              | 55.2%          | 71.4%            | 69.9%            | 66.0%             |
| Trustmark Q (0.95) | RivaGAN            | LC[131,32,37] | series   | 0.1  | 32                 | 99.2%    | 40.7              | 1.0              | 98.9%              | 55.2%          | 69.7%            | 67.4%            | 64.5%             |
| Trustmark Q (0.95) | RivaGAN            | LC[131,32,37] | series   | 0.2  | 32                 | 99.2%    | 40.9              | 1.0              | 98.5%              | 53.2%          | 67.5%            | 65.7%            | 62.7%             |
| Trustmark Q (0.95) | RivaGAN            | LC[131,32,37] | series   | 0.3  | 32                 | 99.2%    | 41.1              | 1.1              | 99.0%              | 52.2%          | 67.4%            | 66.8%            | 62.8%             |
| Trustmark Q (0.95) | RivaGAN            | LC[131,32,37] | series   | 0.4  | 32                 | 98.7%    | 41.3              | 1.2              | 98.2%              | 51.0%          | 66.4%            | 63.9%            | 61.7%             |
| Trustmark Q (0.95) | RivaGAN            | LC[131,32,37] | series   | 0.5  | 32                 | 97.9%    | 41.5              | 1.2              | 97.7%              | 50.2%          | 64.4%            | 63.0%            | 55.7%             |
| Trustmark Q (0.95) | RivaGAN            | LC[131,32,37] | series   | 0.6  | 32                 | 97.4%    | 41.8              | 1.3              | 97.5%              | 46.7%          | 61.9%            | 60.6%            | 56.0%             |
| Trustmark Q (0.95) | RivaGAN            | LC[131,32,37] | series   | 0.7  | 32                 | 96.7%    | 42.0              | 1.5              | 96.5%              | 45.8%          | 61.3%            | 58.1%            | 53.9%             |
| Trustmark Q (0.95) | RivaGAN            | LC[131,32,37] | series   | 0.8  | 32                 | 95.6%    | 42.2              | 1.6              | 95.6%              | 44.8%          | 57.6%            | 57.6%            | 52.5%             |
| Trustmark Q (0.95) | RivaGAN            | LC[131,32,37] | series   | 0.9  | 32                 | 94.4%    | 42.5              | 1.8              | 94.3%              | 43.1%          | 56.4%            | 54.3%            | 48.8%             |
| Trustmark Q (0.95) | RivaGAN            | LC[131,32,37] | series   | 1    | 32                 | 92.8%    | 42.7              | 1.9              | 93.3%              | 40.3%          | 53.4%            | 51.7%            | 48.9%             |
| Trustmark Q (0.95) | RivaGAN            | LC[131,32,37] | series   | 1.1  | 32                 | 91.3%    | 42.9              | 2.1              | 92.0%              | 41.6%          | 51.6%            | 50.3%            | 47.4%             |
| Trustmark Q (0.95) | RivaGAN            | LC[131,32,37] | series   | 1.2  | 32                 | 89.7%    | 43.2              | 2.2              | 90.0%              | 36.8%          | 50.3%            | 47.3%            | 45.1%             |
| Trustmark Q (0.95) | RivaGAN            | LC[131,32,37] | series   | -    | 32                 | 99.9%    | 38.0              | 1.1              | 100.0%             | 59.6%          | 81.3%            | 77.5%            | 75.3%             |
| Trustmark Q (0.95) | RivaGAN            | -             | series   | 0.5  | 132                | 17.3%    | 41.5              | 1.2              | 20.0%              | 3.8%           | 6.1%             | 5.1%             | 4.4%              |
| Trustmark Q (0.95) | RivaGAN            | -             | series   | -    | 132                | 67.3%    | 38.0              | 1.1              | 66.1%              | 16.8%          | 24.6%            | 22.5%            | 18.8%             |
| Trustmark Q (0.95) | RoSteALS           | -             | series   | 0.5  | 200                | 1.1%     | 36.8              | 2.8              | 0.3%               | 0.0%           | 0.0%             | 0.0%             | 0.0%              |
| Trustmark Q (0.95) | RoSteALS           | -             | series   | -    | 200                | 14.5%    | 30.8              | 3.4              | 7.5%               | 4.4%           | 0.0%             | 0.0%             | 0.0%              |
| Trustmark Q (0.95) | SSL (42dB,30bits)  | -             | series   | 0.5  | 130                | 35.5%    | 42.3              | 1.2              | 33.4%              | 15.9%          | 14.7%            | 14.5%            | 12.6%             |
| Trustmark Q (0.95) | SSL (42dB,30bits)  | -             | series   | -    | 130                | 85.4%    | 39.0              | 1.1              | 83.3%              | 45.8%          | 54.8%            | 49.5%            | 44.5%             |
| Trustmark Q (0.95) | Trustmark B (0.95) | -             | parallel | 0.5  | 200                | 0.0%     | 43.1              | 2.1              | 0.0%               | 0.0%           | 0.0%             | 0.0%             | 0.0%              |
| Trustmark Q (0.95) | Trustmark B (0.95) | -             | parallel | -    | 200                | 0.0%     | 43.1              | 2.1              | 0.0%               | 0.0%           | 0.0%             | 0.0%             | 0.0%              |
| Trustmark Q (0.95) | Trustmark B (0.95) | -             | series   | 0.5  | 200                | 0.0%     | 41.9              | 2.2              | 0.0%               | 0.0%           | 0.0%             | 0.0%             | 0.0%              |
| Trustmark Q (0.95) | Trustmark B (0.95) | -             | series   | -    | 200                | 0.0%     | 38.7              | 2.2              | 0.0%               | 0.0%           | 0.0%             | 0.0%             | 0.0%              |
| Trustmark Q (0.95) | Trustmark Q (0.95) | -             | parallel | 0.5  | 200                | 0.0%     | 42.9              | 2.3              | 0.0%               | 0.0%           | 0.0%             | 0.0%             | 0.0%              |
| Trustmark Q (0.95) | Trustmark Q (0.95) | -             | parallel | -    | 200                | 0.0%     | 42.9              | 2.3              | 0.0%               | 0.0%           | 0.0%             | 0.0%             | 0.0%              |
| Trustmark Q (0.95) | Trustmark Q (0.95) | -             | series   | 0.5  | 200                | 0.0%     | 42.5              | 2.3              | 0.0%               | 0.0%           | 0.0%             | 0.0%             | 0.0%              |
| Trustmark Q (0.95) | Trustmark Q (0.95) | -             | series   | -    | 200                | 0.0%     | 39.0              | 2.4              | 0.0%               | 0.0%           | 0.0%             | 0.0%             | 0.0%              |
| Trustmark Q (1.00) | -                  | LC[100,32,25] | -        | -    | 32                 | 99.9%    | 42.1              | 2.4              | 99.8%              | 71.3%          | 92.0%            | 91.1%            | 90.1%             |
